# Supplementary material for: A deep-learning search for technosignatures of 820 nearby stars
Source: arXiv:2301.12670 source file (2023-01-30)
Supplement: Supplementary file 1 [file main-supps.tex]

%\documentclass[fleqn,10pt]{wlscirep}
%\usepackage[utf8]{inputenc}
%\usepackage[T1]{fontenc}
%\usepackage{bm}
%\usepackage{siunitx}

%\title{Supplementary Materials}

\setcounter{figure}{0}

\thispagestyle{empty}

%\begin{document}

\section*{}

\subsection*{}

\subsection*{}

\begin{figure}[hbt]

  \centering
  \includegraphics[width=\textwidth]{SuppFigure1}
  \caption{}
\end{figure}

\begin{figure}[hbt]
\centering
  \includegraphics[width=0.6\textwidth]{SuppFigure2}
  \caption{}
\end{figure}

\begin{figure}[hbt]
\centering
  \includegraphics[width=0.6\textwidth]{SuppFigure3}
  \caption{}
\end{figure}

%\end{document}
